# Supplementary material for: Synthetic control of structure and conduction properties in Na-Y-Zr-Cl solid electrolytes
Source: arXiv:2208.07823 source file (2022-08-16)
Supplement: Supplementary file 1 [file Supplementary_information.pdf]

# —Supplementary Information— Synthetic control of structure and conduction properties in Na-Y-Zr-Cl solid electrolytes

Elias Sebti[1,2], Ji Qi[3], Peter M. Richardson[1], Phillip Ridley[3], Erik A. Wu[3], Swastika Banerjee[3], Raynald Giovine[1,2], Ashley Cronk[3], So-Yeon Ham[3], Ying Shirley Meng*[3,4], Shyue Ping Ong*[3], and Raphaële J. Clément*[1,2]

[1]*Materials Department, University of California, Santa Barbara, California 93106, United States*

[2]*Materials Research Laboratory, University of California, Santa Barbara, California 93106, United States*

[3]*Department of NanoEngineering, University of California San Diego, 9500 Gilman Dr., La Jolla, San Diego, California 92093, United States*

[4]*Pritzker School of Molecular Engineering, University of Chicago, Chicago, IL, USA*

# Contents


**Sec. S1** **XRD Patterns Obtained on $Na_2ZrCl_6$ Samples** **S4**

**Sec. S2** **Le Bail Refinement of Slow Cooled and Twice Ball Milled $Na_2ZrCl_6$ XRD Patterns** **S5**

**Sec. S3** **Simultated $^{23}Na$ NMR Spectrum of $Na_2ZrCl_6$** **S6**

**Sec. S4** **$^{23}Na$ EXSY on Twice Ball Milled $Na_2ZrCl_6$** **S7**

**Sec. S5** **Fits of the $^{23}Na$ VT-NMR Data Acquired on Twice Ball Milled $Na_2ZrCl_6$** **S8**

**Sec. S6** **$^{23}Na$ VT-NMR on Quenched $Na_2ZrCl_6$** **S10**

**Sec. S7** **XRD Patterns Obtained on $Na_3YCl_6$ Samples** **S11**

**Sec. S8** **SEM of $Na_3YCl_6$** **S12**

**Sec. S9** **Simultated $^{23}Na$ NMR Spectrum of $Na_3YCl_6$** **S13**

**Sec. S10** **$^{23}Na$ EXSY on Twice Ball Milled $Na_3YCl_6$** **S14**

**Sec. S11** **$^{23}Na$ VT-NMR on Quenched $Na_3YCl_6$** **S15**

**Sec. S12** **Microstructure Evolution of Quenched $Na_3YCl_6$ upon a 134 °C Heat Treatment** **S16**

**Sec. S13** **Bond Valence Sum Maps of $Na_2ZrCl_6$ and $Na_3YCl_6$ Polymorphs** **S17**

**Sec. S14** **Le Bail Refinement of Slow Cooled $Na_{2.25}Y_{0.25}Zr_{0.75}Cl_6$ XRD Pattern** **S18**

**Sec. S15** **Raman of $Na_{2.25}Y_{0.25}Zr_{0.75}Cl_6$** **S19**

**Sec. S16** **Energetics of Enumerated $Na_{2.25}Y_{0.25}Zr_{0.75}Cl_6$ Supercells** **S20**

**Sec. S17** **$^{23}Na$ EXSY of twice ball milled $Na_{2.25}Y_{0.25}Zr_{0.75}Cl_6$** **S21**

**Sec. S18** **Cross-sectional SEM of $Na_{2.25}Y_{0.25}Zr_{0.75}Cl_6$ Pellets** **S22**

**Sec. S19** **Improvement of Reliability of MTP with Active Learning** **S23**

**Sec. S20** **Simulated Evolution of Na Octahedral Site Occupancies in $Na_{2.25}Y_{0.25}Zr_{0.75}Cl_6$** **S24**

**Sec. S21** **Simulated Na Motion at 500 K in $Na_{2.25}Y_{0.25}Zr_{0.75}Cl_6$** **S25**

**Sec. S22** **Simulated Cl Motion at 400 K in $Na_{2.25}Y_{0.25}Zr_{0.75}Cl_6$** **S26**

**Sec. S23** **Evolution of Twice Ball Milled $Na_{2.25}Y_{0.25}Zr_{0.75}Cl_6$ EIS-derived Conductivity** **S27**

**Sec. S24** **Metastability of the Twice Ball Milled $Na_{2.25}Y_{0.25}Zr_{0.75}Cl_6$ Structure** **S28**

**Sec. S25** **Parameter Convergence for NMR CASTEP Calculations** **S29**

**Sec. S26** **$^{23}$Na Chemical Shift Calibration Curve for Analysis of NMR CASTEP Calculation Results** **S30**

# Sec. S1 XRD Patterns Obtained on $Na_2ZrCl_6$ Samples

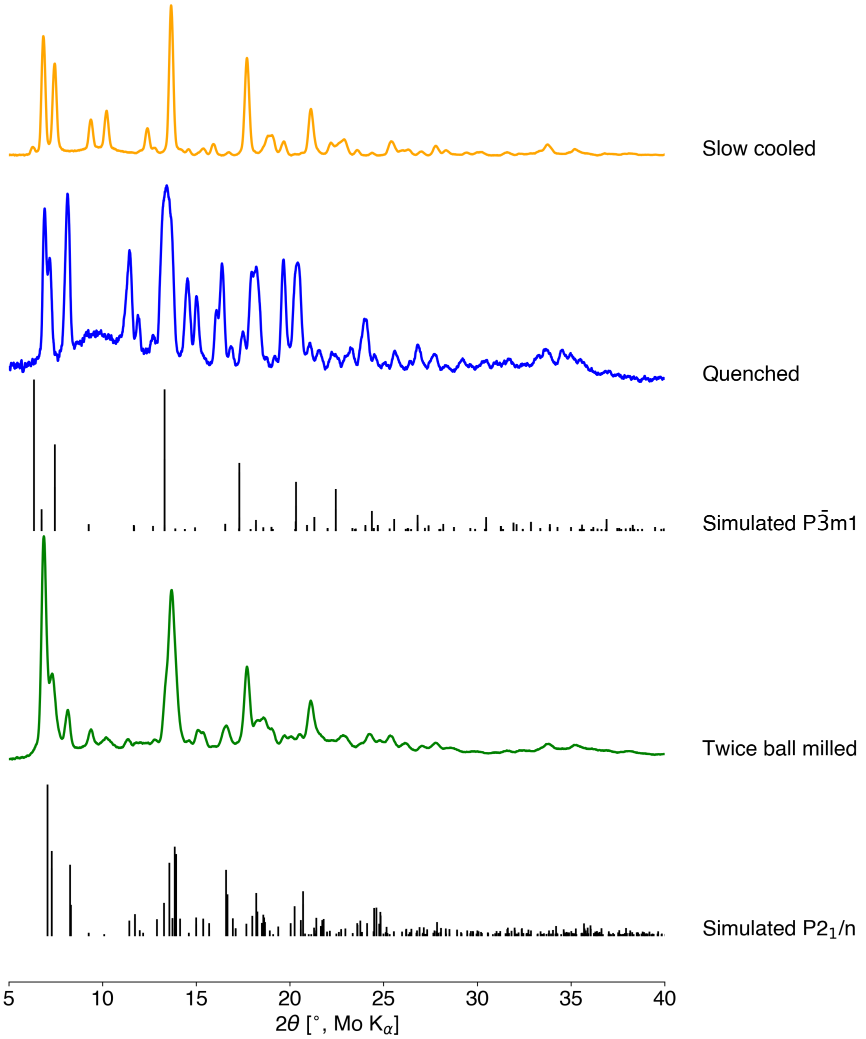


**Figure S1: Comparison of simulated XRD patterns for lowest energy P$\bar{3}$m1 and P$2_1$/n $Na_2ZrCl_6$ enumerated model structures obtained from DFT and patterns obtained on the slow cooled, quenched, and twice ball milled samples. Quenched and twice ball milled patterns are reproduced from[1].**

# Sec. S2 Le Bail Refinement of Slow Cooled and Twice Ball Milled $Na_2ZrCl_6$ XRD Patterns

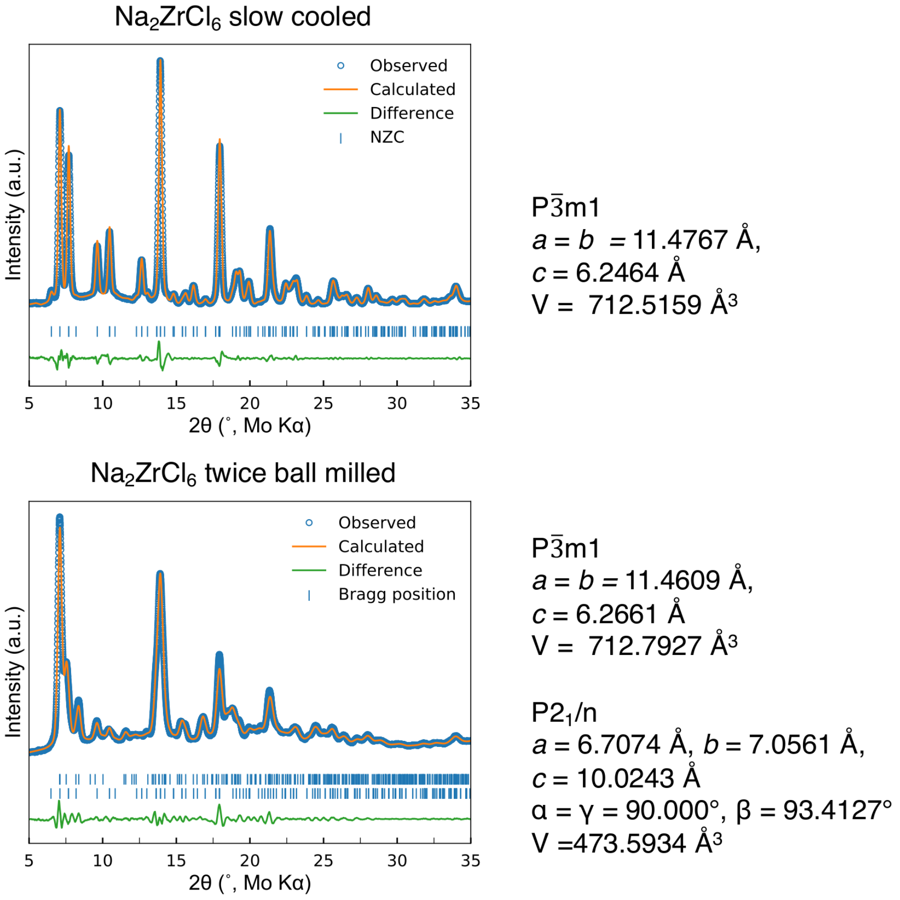


**Figure S2:** Le Bail refinement conducted on the XRD patterns of slow cooled (top) and twice ball milled (bottom) $Na_2ZrCl_6$ samples. The twice ball milled pattern is reproduced from[1].

## Sec. S3 Simultated $^{23}$Na NMR Spectrum of $Na_2ZrCl_6$

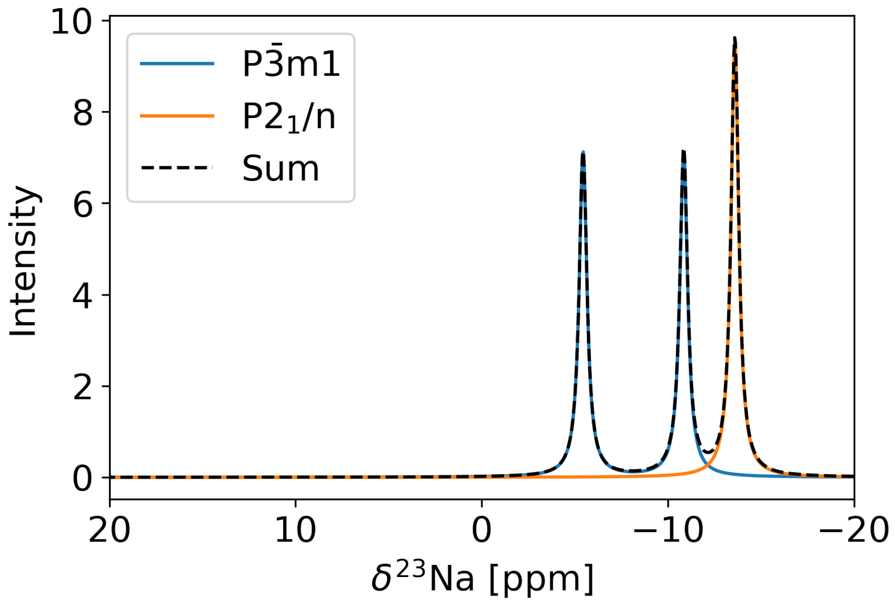


**Figure S3: Reconstruction of the $^{23}$Na NMR resonances expected for the $Na_2ZrCl_6$ P$\bar{3}$m1 and P$2_1$/n polymorphs using Lorentzian lineshapes centered at the calibrated chemical shift values obtained from NMR CASTEP simulations. For each computed shift, a signal linewidth of 0.5 ppm was used to best replicate experimentally-observed lineshapes across preparation methods.**

## Sec. S4 $^{23}$Na EXSY on Twice Ball Milled $Na_2ZrCl_6$

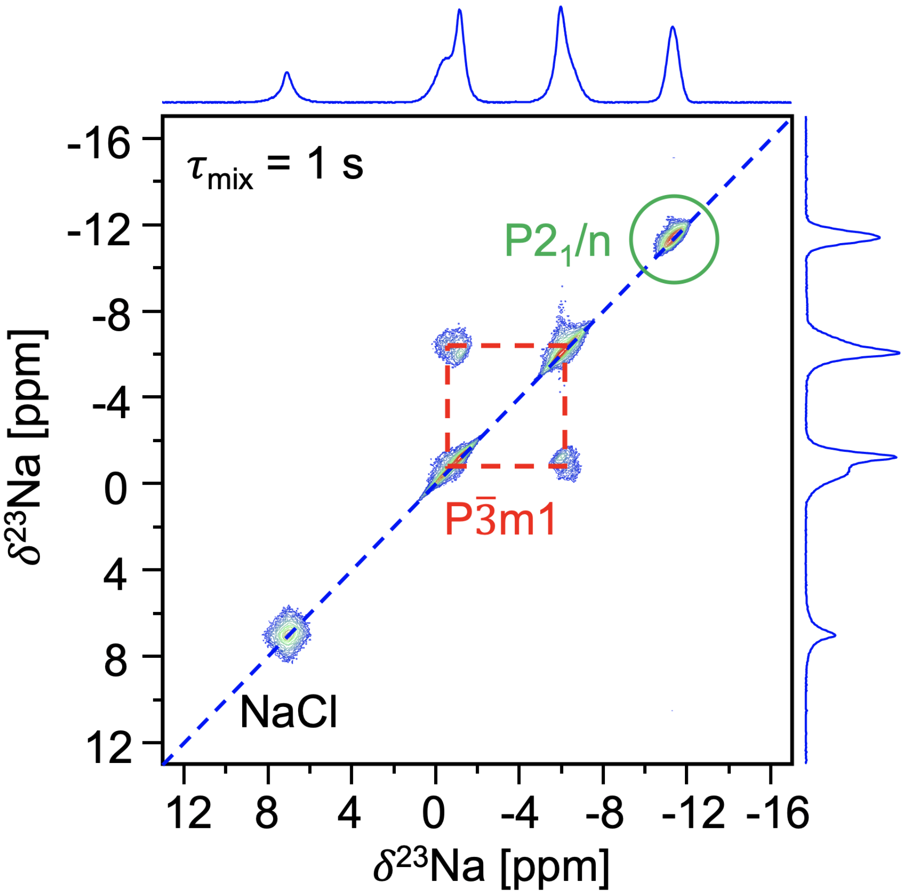


**Figure S4: $^{23}$Na 2D EXSY spectrum obtained on twice ball milled $Na_2ZrCl_6$ at 55 °C (328 K) and using a 1 s mixing time ($\tau_{mix}$). The 1D spectrum collected on this sample is projected on the right hand side and at the top of the 2D spectrum. All spectra were acquired at 18.8 T using a 3.2 mm HX probe at a 10 kHz MAS spinning speed. Longitudinal relaxation times ($T_1$) for the two phases of $Na_2ZrCl_6$ were around 4 s, allowing minimal signal loss during the 1 s of mixing time.**

## Sec. S5 Fits of the $^{23}$Na VT-NMR Data Acquired on Twice Ball Milled $Na_2ZrCl_6$

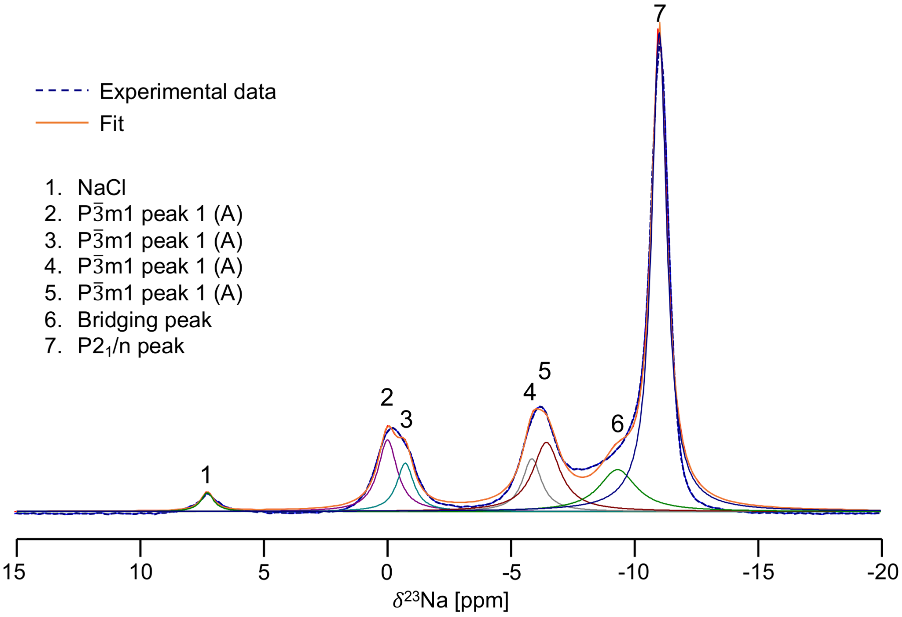


**Figure S5: Example fit of a $^{23}$Na MAS-NMR spectrum measured at 45 °C on twice ball milled $Na_2ZrCl_6$. The spectrum was acquired at 18.8 T with a 10 kHz spinning speed.**

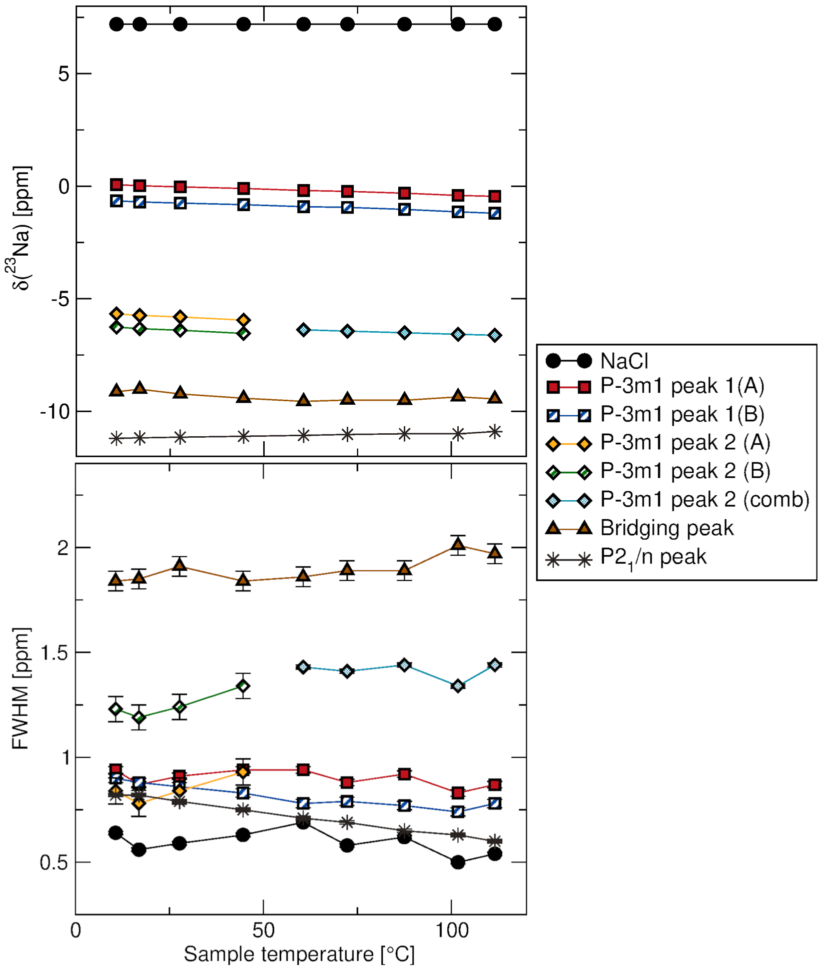


**Figure S6: Evolution of the (a) isotropic shift ($\delta(^{23}Na)$) and (b) full width half max (FWHM) obtained from fits of the VT-NMR $^{23}$Na MAS-NMR spectra acquired on twice ball milled $Na_2ZrCl_6$ between 11 and 112 °C. All lineshapes were fitted using a Lorentzian function. Above 50 °C, a single peak was required to appropriately fit the P$\bar{3}$m1 peak 2. The NaCl resonance was fixed at 7.2 ppm to serve as an internal reference. Error bars for both sets of fitting parameters (excluding the P$\bar{3}$m1 combined peak 2) were calculated from the standard deviation of values obtained from five fits of the spectrum measured at 44.6 °C, starting from different initial guesses. Error bars for the P$\bar{3}$m1 combined peak 2 were calculated at 102°C. The error bar on the fitted isotropic shifts is negligible and within the size of the labels used in this figure. Fluctuations in the FWHM values for the NaCl resonance are attributed to the small NaCl phase fraction in the sample which made the lineshape more subject to noise during each acquisition.**

# Sec. S6 $^{23}$Na VT-NMR on Quenched $Na_2ZrCl_6$

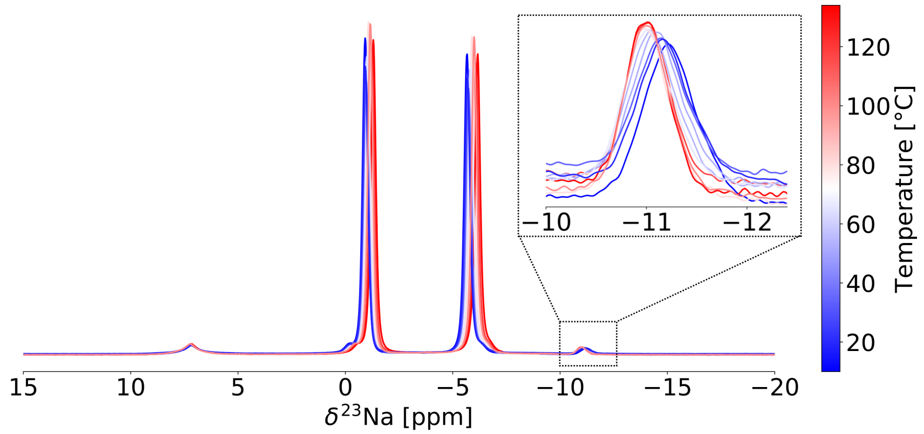


**Figure S7:** **$^{23}$Na VT-NMR of quenched $Na_2ZrCl_6$ measured between 10 °C and 134 °C. Spectra are color-coded using the temperature scale on the right of the plot. The peak at 7.2 ppm corresponds to NaCl. Spectra were obtained at 18.8 T with a 10 kHz MAS spinning speed. An inset of the $P2_1/n$ resonance is provided to highlight the evolution of its isotropic shift with temperature.**

## Sec. S7 XRD Patterns Obtained on $Na_3YCl_6$ Samples

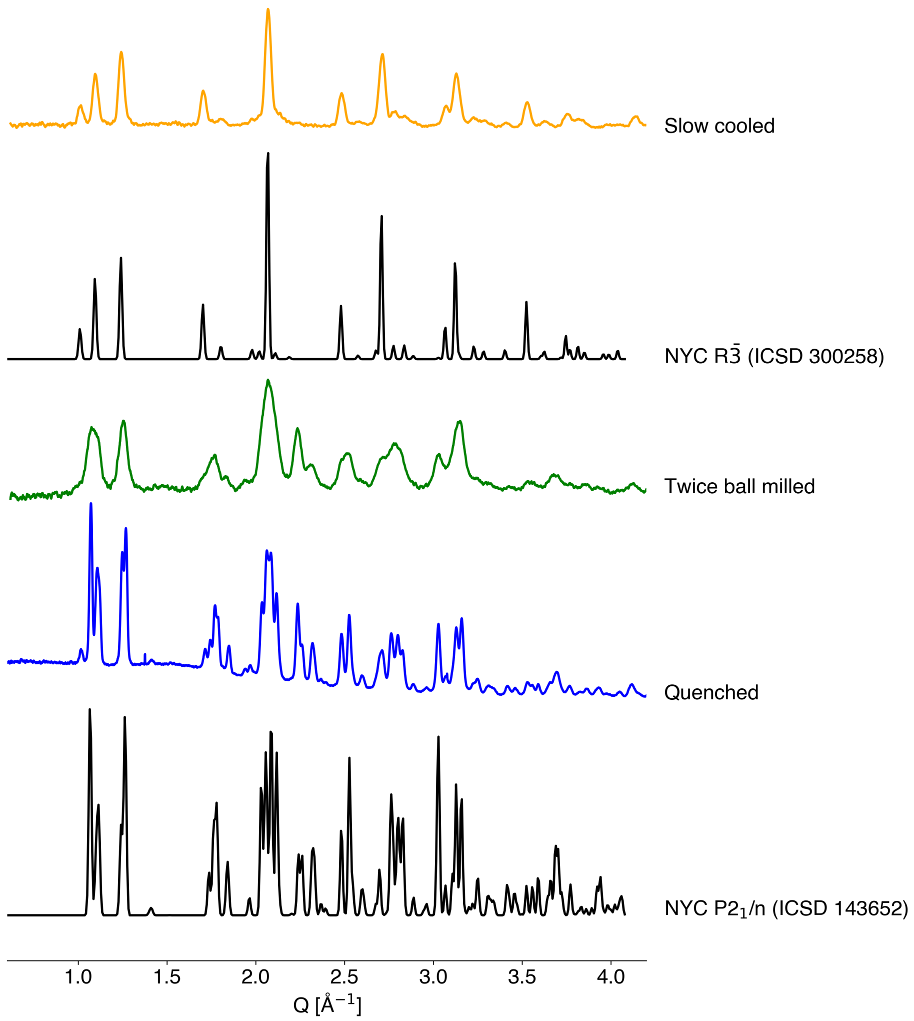


**Figure S8: XRD patterns obtained on slow cooled, twice ball milled, and quenched $Na_3YCl_6$ along with comparisons against simulated patterns for reported structures for each $Na_3YCl_6$ polymorph. Patterns for the quenched and twice ball milled samples are reproduced from[1]. ICSD structures used for the simulated patterns of the $R\bar{3}$ and $P2_1/n$ $Na_3YCl_6$ structures are obtained from[2] and[1], respectively.**

## Sec. S8 SEM of $Na_3YCl_6$

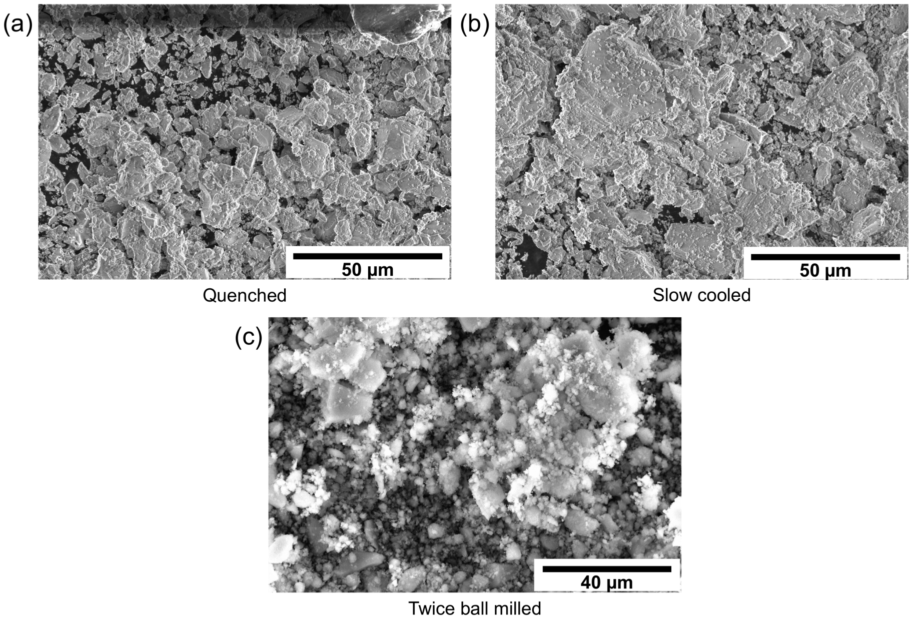


**Figure S9: SEM micrographs obtained on unpressed $Na_3YCl_6$ powders that were prepared by initial ball milling followed by an annealing step and a (a) water bath quenching step (quenched), or (b) a 48 h slow cooling step (slow cooled). (c) After a second ball milling step of the quenched sample (twice ball milled).**

## Sec. S9 Simultated $^{23}$Na NMR Spectrum of $Na_3YCl_6$

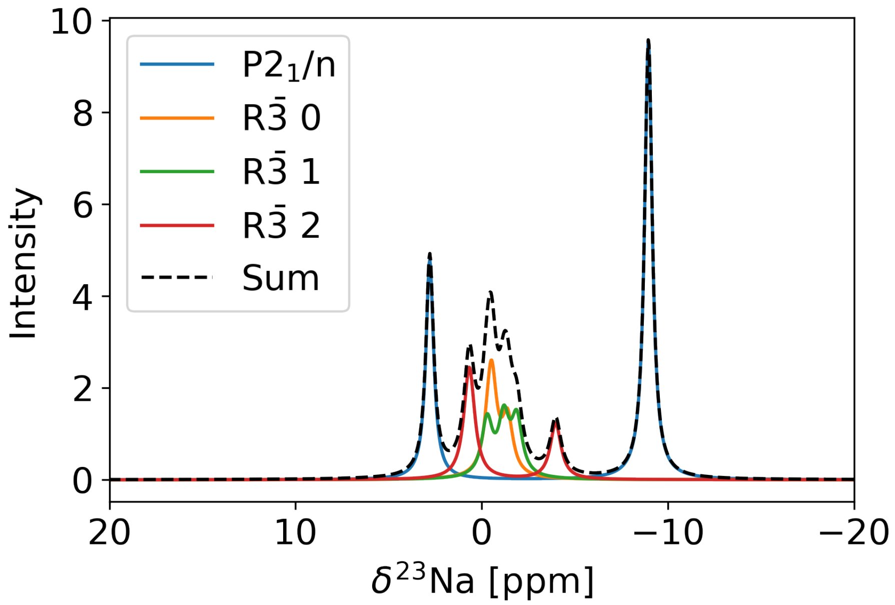


**Figure S10: Reconstruction of the $^{23}$Na NMR resonances expected for the $Na_3YCl_6$ R$\bar{3}$ and P$2_1$/n polymorphs using Lorentzian lineshapes centered at the calibrated chemical shift values obtained from NMR CASTEP simulations and a signal linewidth of 0.7 ppm and 0.5 ppm for the R$\bar{3}$ and P$2_1$/n forms, respectively. Various Na-vacancy orderings were enumerated for the R$\bar{3}$ structure. A larger linewidth value was used for the R$\bar{3}$ as the experimentally observed signal is expected to be an average of the shifts calculated for the various enumerated orderings due to fast Na exchange between individual sites in the R$\bar{3}$ structure on the NMR timescale.**

## Sec. S10 $^{23}$Na EXSY on Twice Ball Milled $Na_3YCl_6$

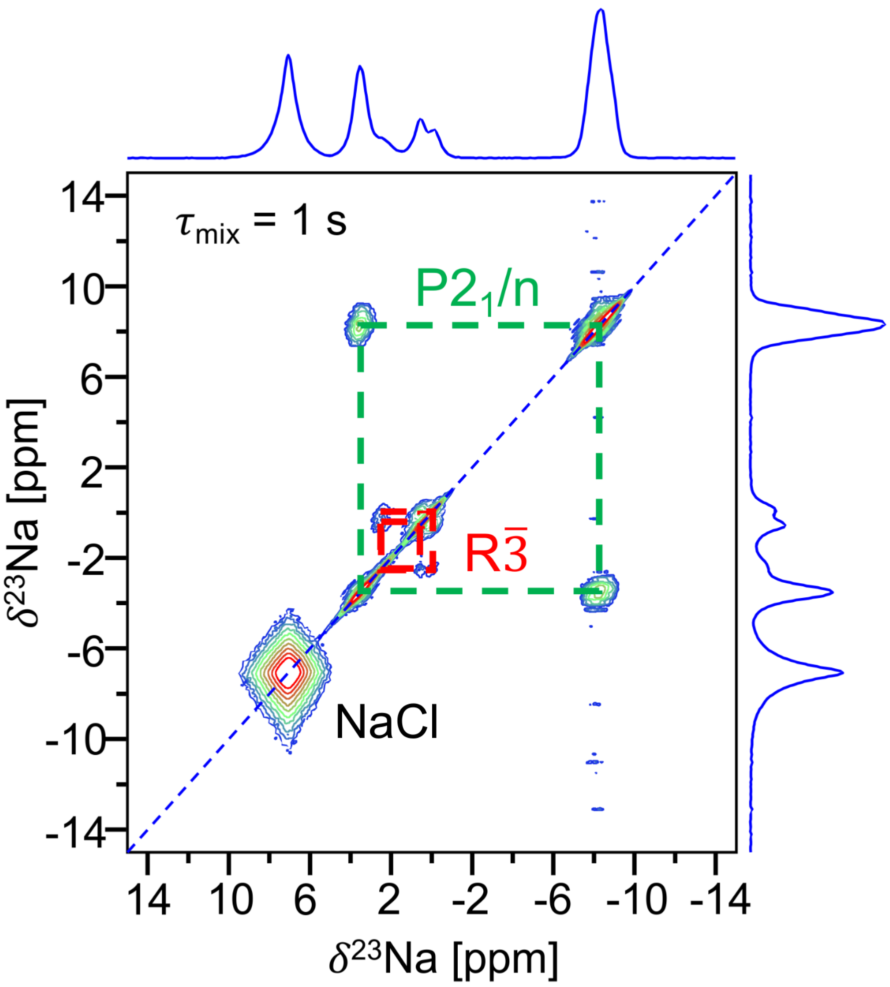


**Figure S11:** $^{23}$Na 2D EXSY spectrum obtained on twice ball milled $Na_3YCl_6$ at 55 °C (328 K) and using a 1 s mixing time ($\tau_{mix}$). The 1D spectrum collected on this sample is projected on the right hand side and at the top of the 2D spectrum. All spectra were acquired at 18.8 T using a 3.2 mm HX probe at a 10 kHz MAS spinning speed. Longitudinal relaxation times ($T_1$) for both $Na_3YCl_6$ phases were on the order of 4 s, allowing minimal signal loss during the 1 s of mixing time.

## Sec. S11 $^{23}$Na VT-NMR on Quenched $Na_3YCl_6$

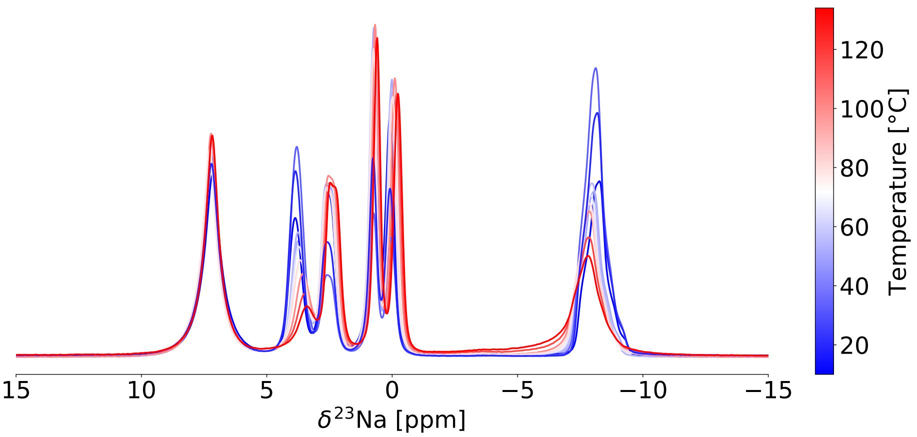


**Figure S12: $^{23}$Na VT-NMR on quenched $Na_3YCl_6$. Spectra are color-coded using the temperature scale on the right of the plot. The peak at 7.2 ppm is NaCl. All spectra were obtained at 18.8 T with a 10 kHz MAS spinning speed.**

## Sec. S12 Microstructure Evolution of Quenched $Na_3YCl_6$ upon a 134 °C Heat Treatment

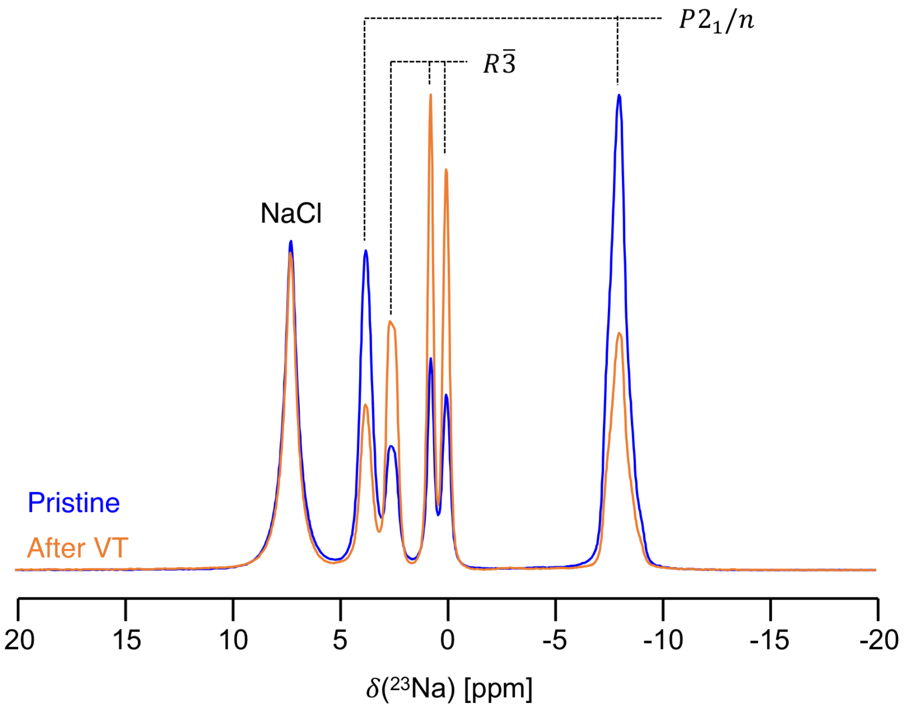


**Figure S13:** $^{23}$**Na MAS-NMR spectra collected at 52 °C (328 K) on quenched $Na_3YCl_6$ before and after VT-NMR measurements. Spectra were acquired at 18.8 T using a 3.2 mm HX probe at a 10 kHz MAS spinning speed. The phase fraction of the R$\bar{3}$ increases after exposure to temperatures up to 134 °C during VT-NMR measurements.**

## Sec. S13 Bond Valence Sum Maps of $Na_2ZrCl_6$ and $Na_3YCl_6$ Polymorphs

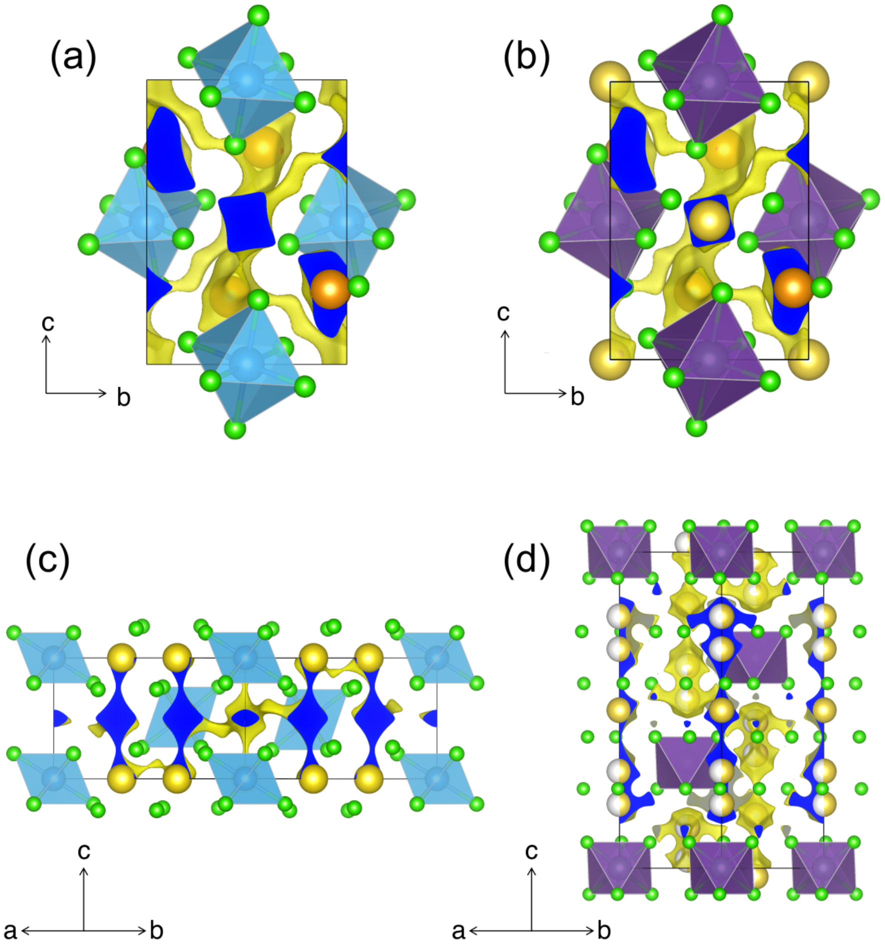


**Figure S14: Bond valence sum maps calculated for the $P2_1/n$ forms of (a) $Na_2ZrCl_6$ and (b) $Na_3YCl_6$, as well as (c) $P\bar{3}m1$ $Na_2ZrCl_6$ and (d) $R\bar{3}$ $Na_3YCl_6$. Color legend: Y is purple, Zr is light blue, Cl is light green, while Na atoms in octahedral or prismatic environments are yellow and orange, respectively. Bond valence maps were calculated with softBV[3] and the visualized isosurface level was set to 0.1.**

## Sec. S14 Le Bail Refinement of Slow Cooled $Na_{2.25}Y_{0.25}Zr_{0.75}Cl_6$ XRD Pattern

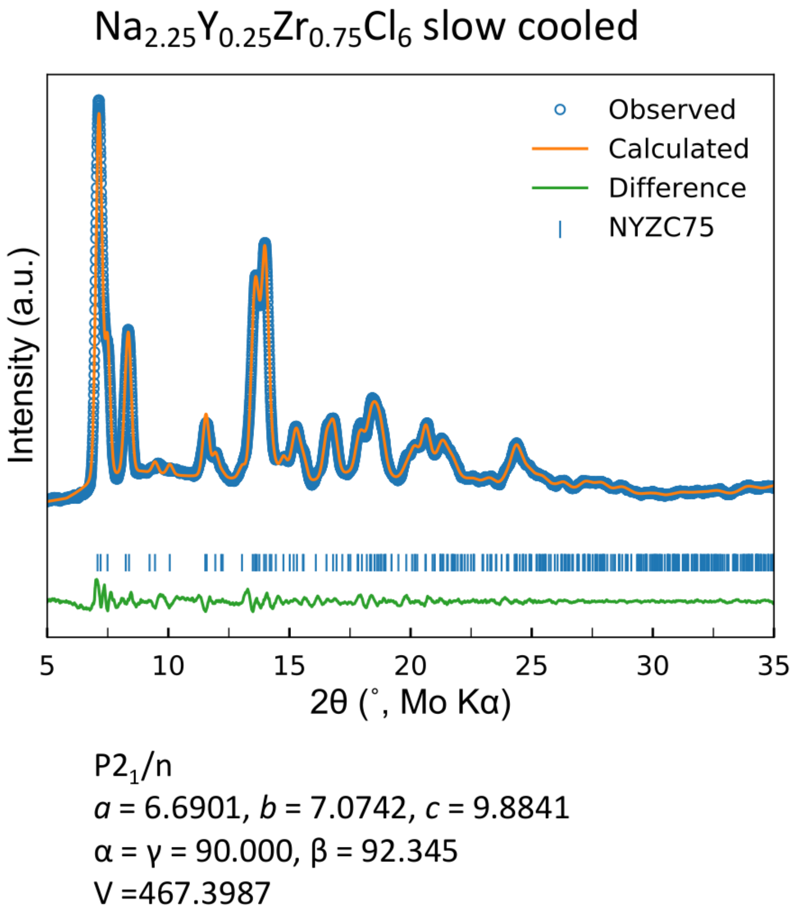


**Figure S15: Le Bail refinement of the XRD pattern obtained for slow cooled $Na_{2.25}Y_{0.25}Zr_{0.75}Cl_6$.**

# Sec. S15 Raman of $Na_{2.25}Y_{0.25}Zr_{0.75}Cl_6$

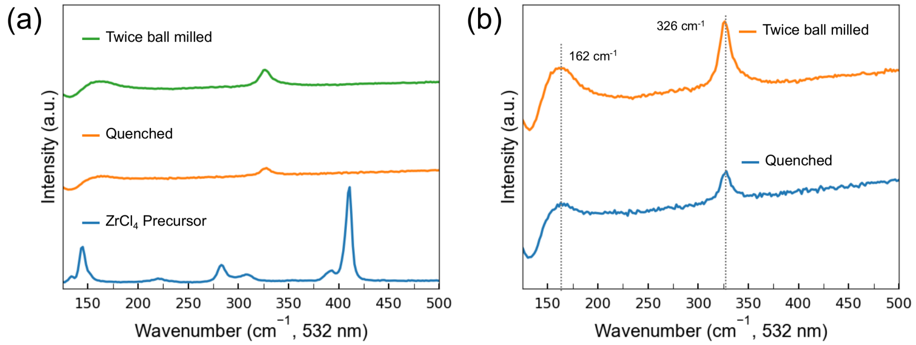


**Figure S16: Raman spectra collected on twice ball milled and quenched $Na_{2.25}Y_{0.25}Zr_{0.75}Cl_6$ samples as well as a $ZrCl_4$ precursor. Spectra were obtained with a 532 nm laser source.**

## Sec. S16 Energetics of Enumerated $Na_{2.25}Y_{0.25}Zr_{0.75}Cl_6$ Supercells

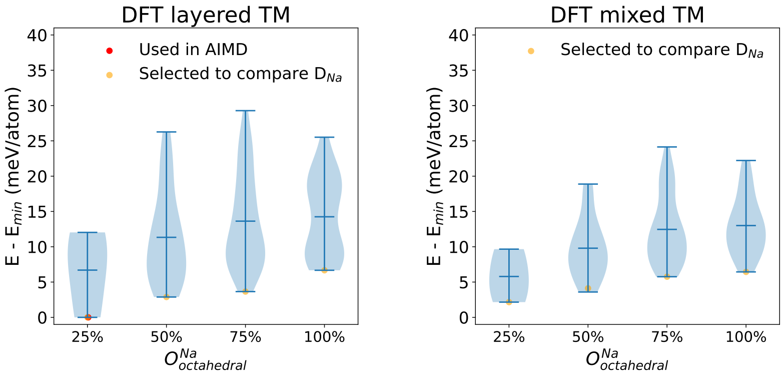


**Figure S17: Energy distribution of the (a) 114 layered-TM and (b) 115 mixed-TM supercells of $Na_{2.25}Y_{0.25}Zr_{0.75}Cl_6$ simulated by DFT.**

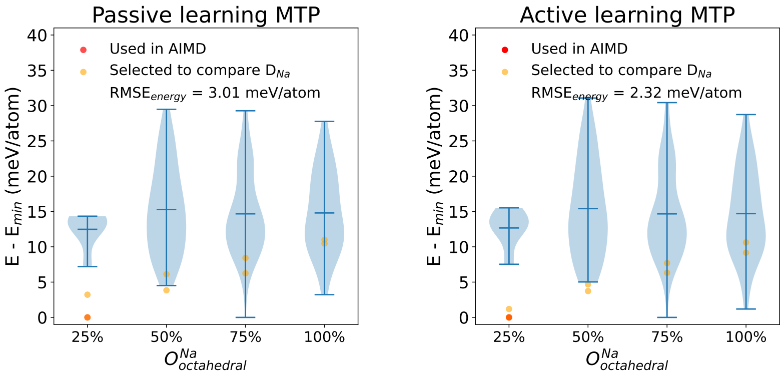


**Figure S18: Energy distribution of the 229 enumerated supercells of $Na_{2.25}Y_{0.25}Zr_{0.75}Cl_6$ by (a) the passive learning MTP and (b) the active learning MTP.**

## Sec. S17 $^{23}$Na EXSY of twice ball milled $Na_{2.25}Y_{0.25}Zr_{0.75}Cl_6$

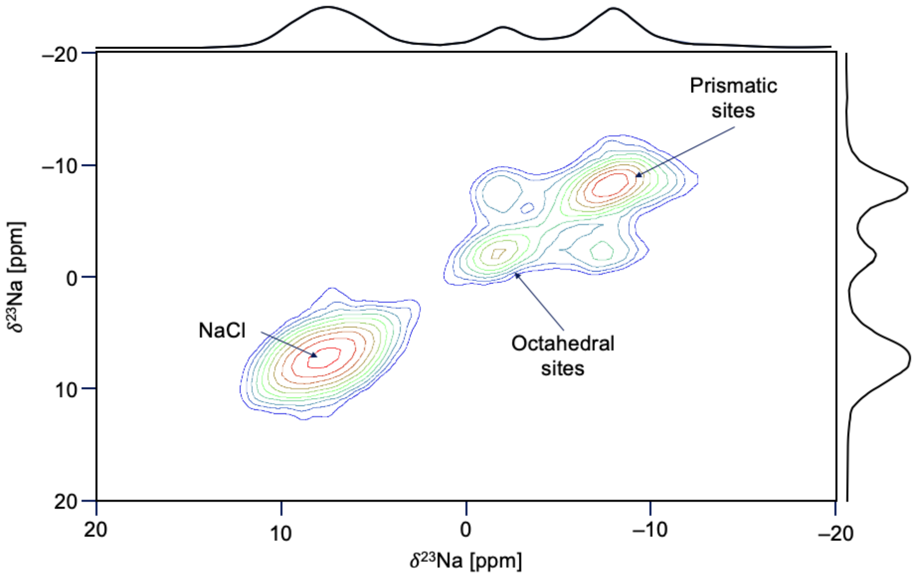


**Figure S19:** **$^{23}$Na EXSY conducted at 55 °C (328 K) on twice ball milled $Na_{2.25}Y_{0.25}Zr_{0.75}Cl_6$. Spectra were acquired at 18.8 T using a 3.2 mm HX probe at a 10 kHz spinning speed with a 50 ms mixing time ($\tau_{mix}$).**

# Sec. S18 Cross-sectional SEM of $Na_{2.25}Y_{0.25}Zr_{0.75}Cl_6$ Pellets

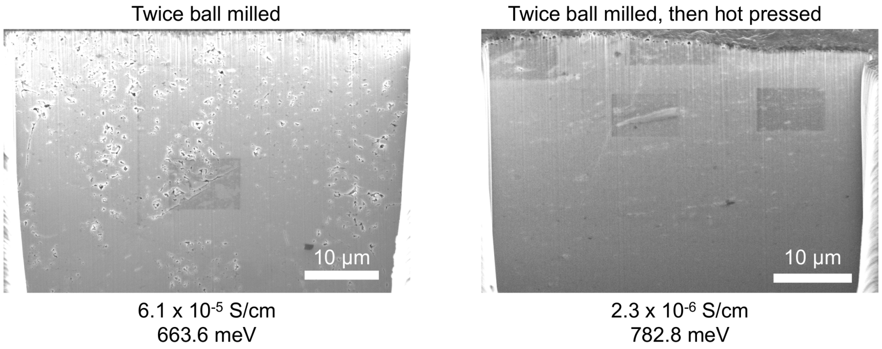


**Figure S20: Cross-sectional SEM micrographs collected on (left) a densified twice ball milled $Na_{2.25}Y_{0.25}Zr_{0.75}Cl_6$ pellet and (right) a hot pressed, twice ball milled $Na_{2.25}Y_{0.25}Zr_{0.75}Cl_6$ pellet. Na-ion conductivities and transport activation energies for each sample are reported below each panel. Hot pressing was conducted at 300 °C under an identical pressure of 370 MPa for 4 hrs. Despite the clear decrease in the void area of the pellet upon hot pressing, Na-ion transport is severely hindered after hot pressing. These findings can be accounted for by changes in the cation distribution within the bulk of twice ball milled NYZC75, as evidenced by the NMR spectra collected before and after the sample was exposed to 111 °C (see Figure S26). It is anticipated that such changes are even more pronounced upon hot pressing at 300 °C, leading to a more significant decrease in Na-ion conduction.**

# Sec. S19 Improvement of Reliability of MTP with Active Learning

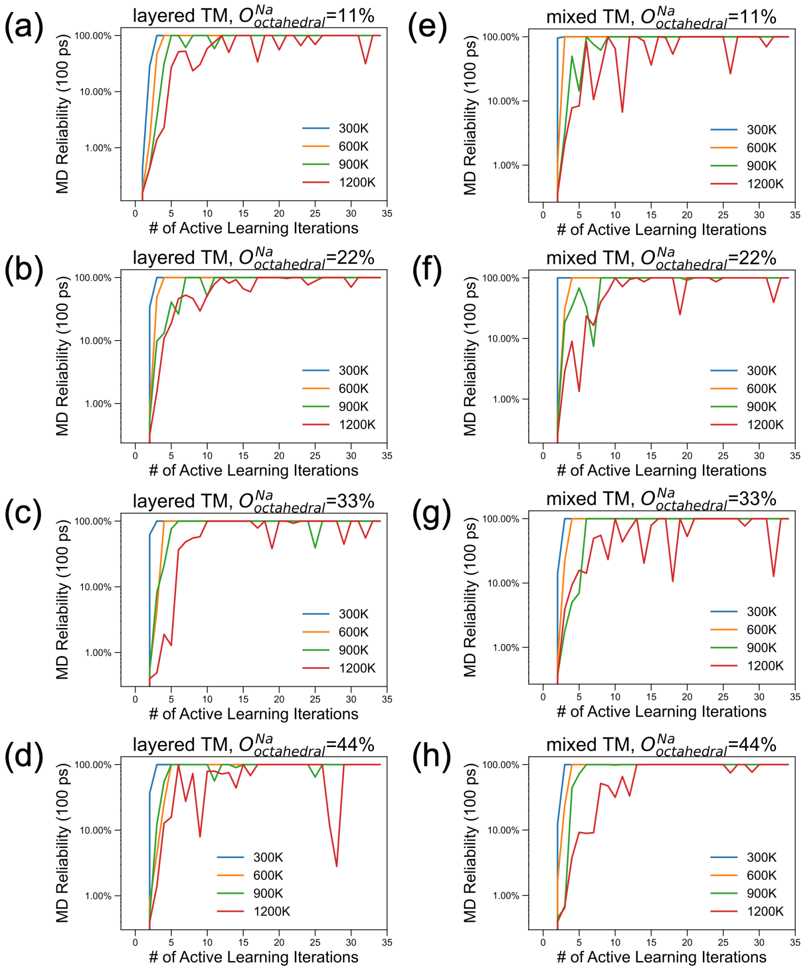


**Figure S21: Improvement of MD reliability for MTP through active learning iterations. The active learning are performed to (a-d) 4 layered-TM structures and (e-h) 4 mixed-TM structures spanning different Na site occupancies. After 34 iterations of active learning, 100% MD reliabilities, i.e., completing 100 ps MD without snapshots having $\gamma$ over 5 were achieved at 300 to 1200 K with 300 K intervals for all the 8 structures.**

# Sec. S20 Simulated Evolution of Na Octahedral Site Occupancies in $Na_{2.25}Y_{0.25}Zr_{0.75}Cl_6$

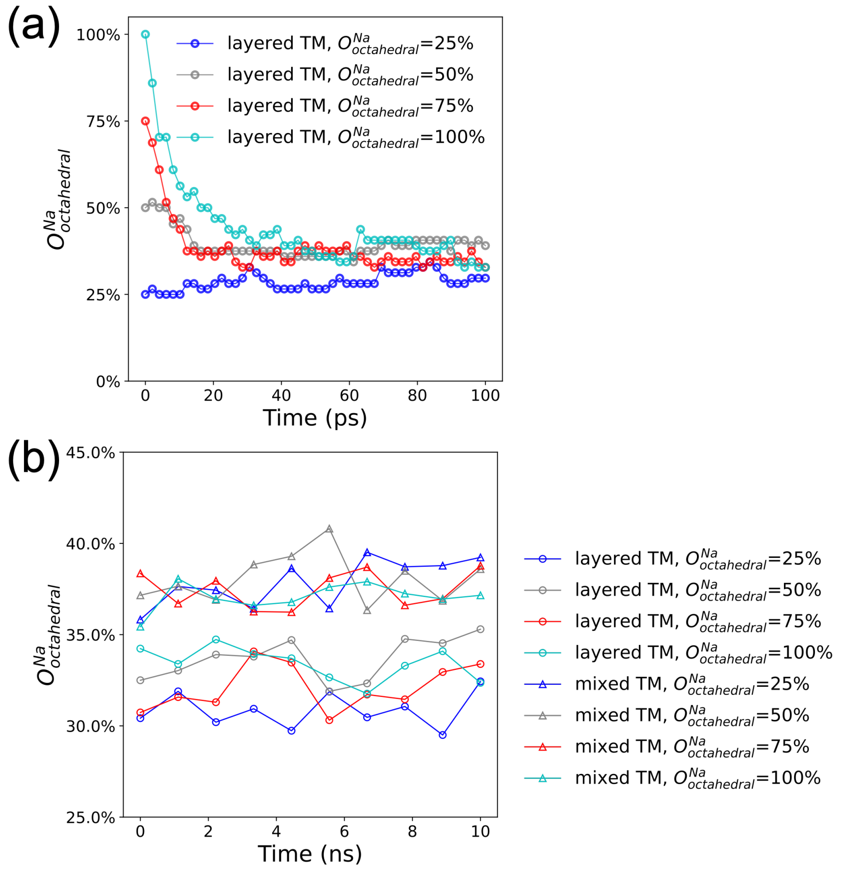


**Figure S22:** (a) Simulated evolution of $O^{Na}_{octahedral}$ in layered-TM structures at the first 100 ps of MD simulations at 400 K. (b) The evolution of equilibrated $O^{Na}_{octahedral}$ in layered-TM and mixed-TM structures in 10 ns of MD simulations at 400 K. Each data point was averaged with 100 trajectory snapshots for better illustration of averaged trend.

## Sec. S21 Simulated Na Motion at 500 K in $Na_{2.25}Y_{0.25}Zr_{0.75}Cl_6$

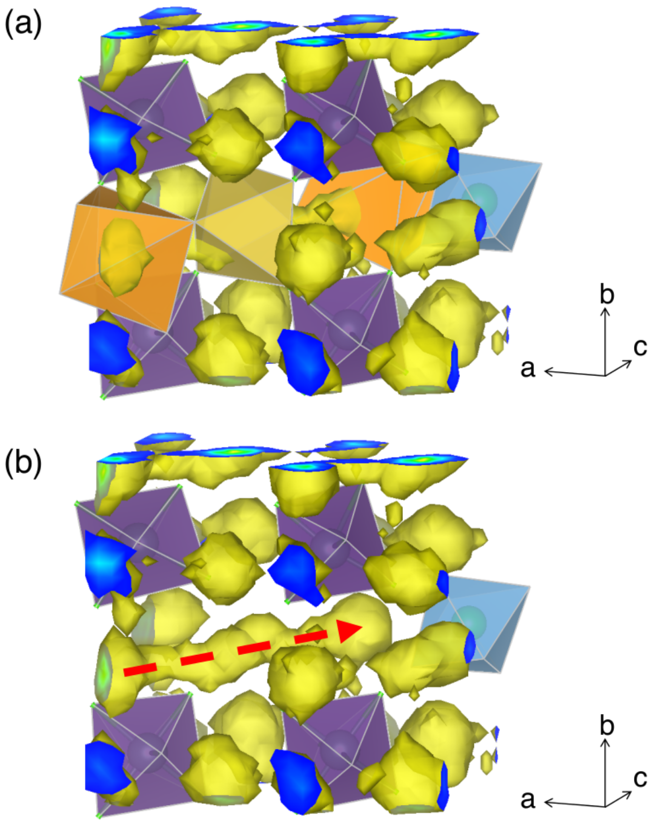


**Figure S23: Plot of the probability density (isosurface value = $6.5\times10^{-5}$) in $Na_{2.25}Y_{0.25}Zr_{0.75}Cl_6$ model supercell simulated by AIMD at 500 K in our previous work[1]. $YCl_6{}^{3-}$ and $ZrCl_6{}^{2-}$ polyhedra are shown in purple and light blue, respectively. Polyhedra for Na prismatic (orange) and octahedral (yellow) sites are displayed in panel (a), and the hopping pathway (red dashed arrow) is highlighted in panel (b). Cl atoms are omitted from the diagram for clarity.**

## Sec. S22 Simulated Cl Motion at 400 K in $Na_{2.25}Y_{0.25}Zr_{0.75}Cl_6$

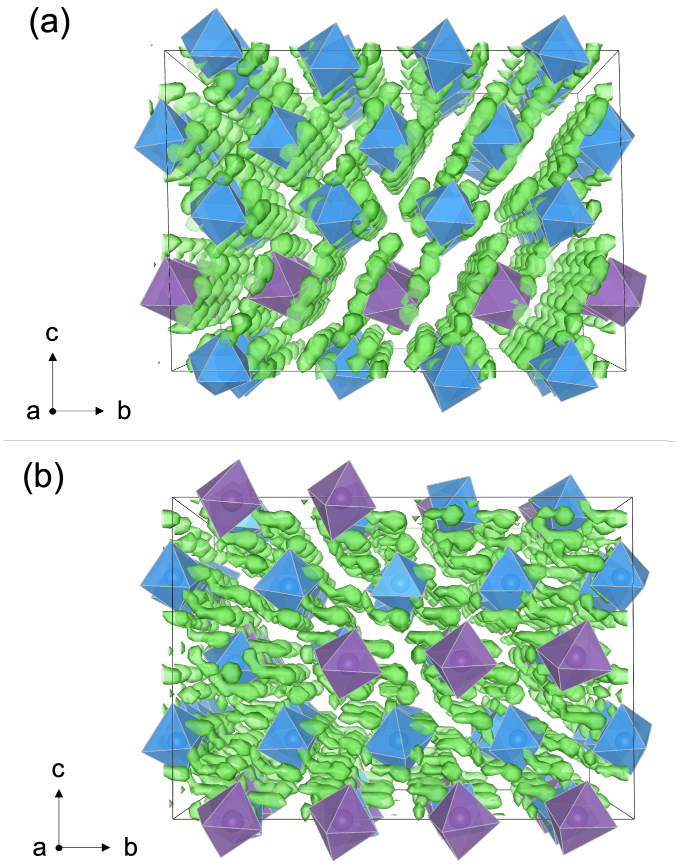


**Figure S24: Plots of the probability density (isosurface value = $3\times10^{-4}$) of $Cl^-$ in (a) layered-TM and (b) mixed-TM structures of $Na_{2.25}Y_{0.25}Zr_{0.75}Cl_6$ simulated by MTP at 400 K. Color legend: Y is purple, Zr is light blue, and Cl is light green. Na is not displayed for visual clarity.**

## Sec. S23 Evolution of Twice Ball Milled $Na_{2.25}Y_{0.25}Zr_{0.75}Cl_6$ EIS-derived Conductivity

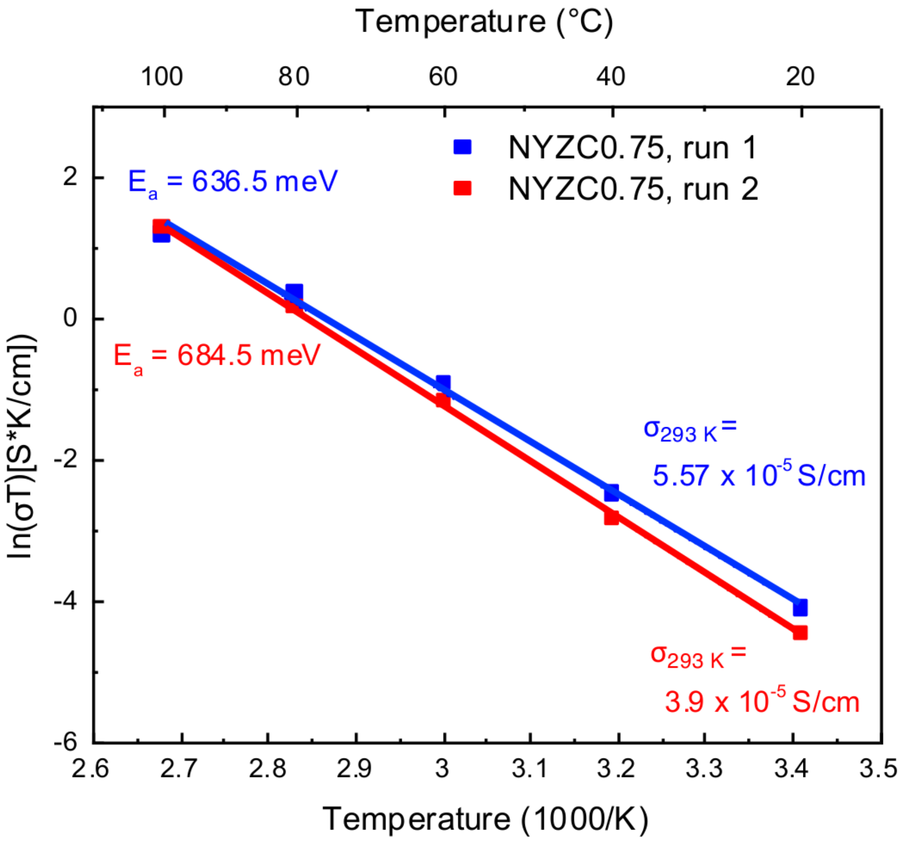


**Figure S25: Successive temperature ramp EIS measurements on twice ball milled $Na_{2.25}Y_{0.25}Zr_{0.75}Cl_6$. Impedance spectra were obtained at regular 20 °C increments as the temperature of the sample was increased from 20 °C to 100 °C. The sample temperature was then decreased back down to 20 °C and the process was repeated to assess the impact of heating on the sample conductivity.**

## Sec. S24 Metastability of the Twice Ball Milled $Na_{2.25}Y_{0.25}Zr_{0.75}Cl_6$ Structure

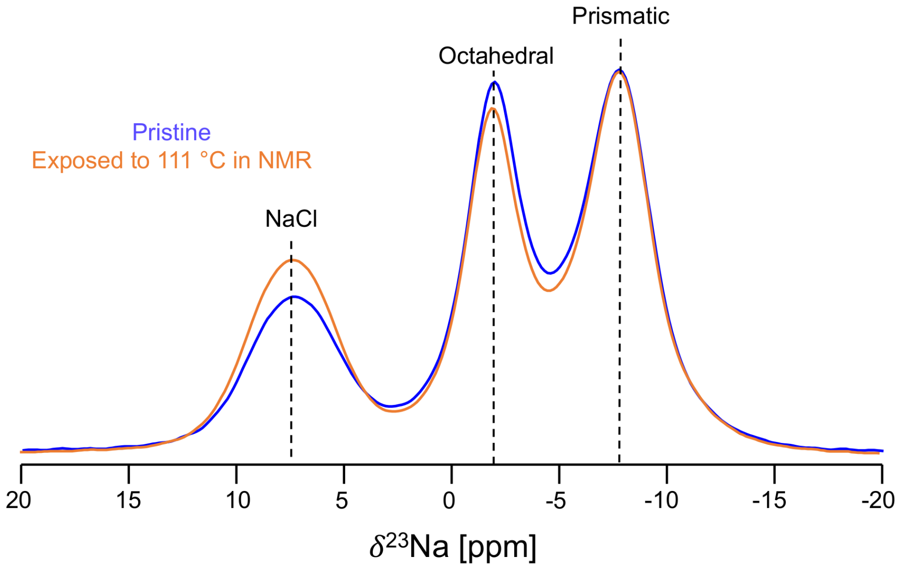


**Figure S26:** $^{23}$**Na MAS-NMR obtained at 55 °C on a twice ball milled $Na_{2.25}Y_{0.25}Zr_{0.75}Cl_6$ sample in its pristine state and after overnight exposure to temperatures up 111 °C. Spectra were acquired at 18.8 T with a 12 kHz spinning speed. Octahedral site occupancy decreases while the NaCl impurity over the course of the high temperature exposure.**

## Sec. S25 Parameter Convergence for NMR CASTEP Calculations

**Table S1: NMR CASTEP calculations parameters. For geometry optimization calculations, plane wave energy cutoffs (in Ry) and $k$-point grids were selected based on a 0.5 meV atom$^{-1}$ convergence criterion for single point energy calculations. An isotropic chemical shielding constant convergence criterion of 0.5 ppm was used for $^{23}$Na NMR parameters. For consistency, all NMR parameter calculations used an 80 Ry plane wave energy cutoff.**

| | Geometry optimization | | NMR calculations | |
|---|---|---|---|---|
| **Compound** | **$k$-point grid** | **cutoff** | **$k$-point grid** | **cutoff** |
| NaCl | 4×4×4 | 50 | 4×4×4 | 80 |
| $Na_2O$ | 4×4×4 | 80 | 4×4×4 | 80 |
| $Na_2S$ | 4×4×4 | 60 | 4×4×4 | 80 |
| $Na_2S_2$ | 6×6×3 | 70 | 8×8×4 | 80 |
| NaBr | 4×4×4 | 60 | 4×4×4 | 80 |
| NaF | 4×4×4 | 70 | 4×4×4 | 80 |
| NaOH | 6×2×6 | 70 | 6×2×6 | 80 |
| $Na_2ZrCl_6$, P$\bar{3}$m1 | 3×3×6 | 50 | 3×3×6 | 80 |
| $Na_2ZrCl_6$, P$2_1$/n | 3×3×2 | 50 | 6×6×4 | 80 |
| $Na_3YCl_6$, P$2_1$/n | 3×3×2 | 60 | 4×4×3 | 80 |
| $Na_3YCl_6$, R$\bar{3}$ | 3×3×3 | 60 | 3×3×3 | 80 |
| $Na_{2.25}Y_{0.25}Zr_{0.75}Cl_6$ (1) | 3×3×1 | 50 | 4×4×2 | 80 |
| $Na_{2.25}Y_{0.25}Zr_{0.75}Cl_6$ (2) | 3×3×2 | 50 | 4×4×3 | 80 |

## Sec. S26 $^{23}$Na Chemical Shift Calibration Curve for Analysis of NMR CASTEP Calculation Results

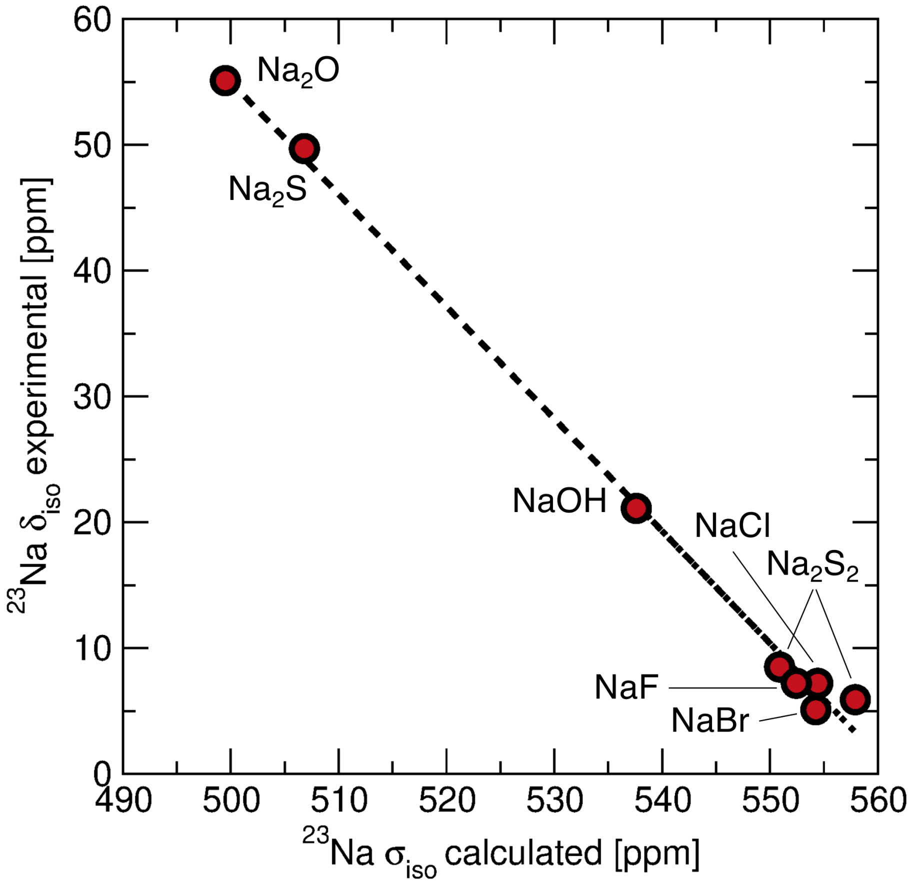


**Figure S27:** **$^{23}$Na NMR semi-empirical calibration curve for converting CASTEP-calculated $\sigma_{iso}$ values to experimentally-relevant $\delta_{iso}$ values.**

**Table S2: NMR CASTEP-calculated $\sigma_{iso}$ and experimentally measured $\delta_{iso}$ for compounds selected for $^{23}$Na NMR calibration curve. $\delta_{\mathrm{iso}}$ is referenced to 1 M NaCl (aq.).**

| **Compound** | **CASTEP $\sigma_{\mathbf{iso}}$** | $\delta_{\mathbf{iso}}$ | **Reference** |
|---|---|---|---|
| NaCl | 554.43 | 7.2 | 4 |
| $Na_2O$ | 499.49 | 55.1 | 5 |
| $Na_2S$ | 506.83 | 49.7 | 6 |
| $Na_2S_2$ | 550.88 | 8.5 | 6 |
| $Na_2S_2$ | 557.91 | 5.9 | 6 |
| NaBr | 554.25 | 5.1 | 4 |
| NaF | 552.44 | 7.2 | 4 |
| NaOH | 537.6 | 21.1 | 4 |

# References


[1] E. A. Wu, S. Banerjee, H. Tang, P. M. Richardson, J.-M. Doux, J. Qi, Z. Zhu, A. Grenier, Y. Li, E. Zhao, G. Deysher, E. Sebti, H. Nguyen, R. Stephens, G. Verbist, K. W. Chapman, R. J. Clément, A. Banerjee, Y. S. Meng and S. P. Ong, *Nat Commun*, 2021, **12**, 1256.

[2] F. Stenzel and G. Meyer, *Z. Anorg. Allg. Chem.*, 1993, **619**, 652–660.

[3] H. Chen, L. L. Wong and S. Adams, *Acta Cryst B*, 2019, **75**, 18–33.

[4] S. F. Dec, G. E. Maciel and J. J. Fitzgerald, *J. Am. Chem. Soc.*, 1990, **112**, 9069–9077.

[5] G. Klösters and M. Jansen, *Solid State Nuclear Magnetic Resonance*, 2000, **16**, 279–283.

[6] G. Mali, M. U. M. Patel, M. Mazaj and R. Dominko, *Chem. Eur. J.*, 2016, **22**, 3355–3360.
